# Supplementary material for: Robust IMMPC: An Offset-free MPC for Rejecting Unknown Disturbances
Source: arXiv:2604.00564 source file (2026-04-01)
Supplement: Supplementary file 1 [file 6_Appendix.tex]

\appendix 
\section{Proof of Theorem \ref{thm:MPC:MainResult}}

\begin{proof}
	To apply the nominal prediction model \eqref{eq:MPC:NominalPredictionModel}, we require the $n_p$-step initialization phase such that the dynamics in Lemma\,\ref{thm:MPC:Model} hold.
	
	\ref{MPC:MPC:Feasibility}  We define a candidate solution at time $t$ using the optimal solution of the previous timestep $t-1$ and using the control input $K_u\xi_{\mathrm{ref},N}^*(t-1)$ at the end.
	From the terminal constraint \eqref{eq:MPC:MPCXTerminal} with the definition of the references \eqref{eq:MPC:MPCXURef} and \eqref{eq:MPC:MPCERef} inserted in \eqref{eq:MPC:Theo:ExtendedXDyn} and \eqref{eq:MPC:Theo:ExtendedEDyn} follows
	\begin{align*}
		\tilde{u}&=[u_{1}^*(t),\ldots,u_{N-1}^*(t),K_u\xi_{\mathrm{ref},N}^*(t)]\\
		\tilde{\xi}&=[\xi_{1}^*(t),\ldots,\xi_{N}^\star(t),(\bar{A}+\bar{B}K_u)\xi_{N}^\star(t)]\\
		\tilde{\xi}_{\mathrm{ref},0} &= \xi_{\mathrm{ref},1}^*(t)
	\end{align*}
	As $\xi(t)\in\xi^*_0(t)\oplus \mathbb{S}$, it follows from \ref{ass:MPC:RPI-Set} that $\xi(t+1)=\xi_1^*(t)\oplus \mathbb{S}$.
	Constraint satisfaction directly follows from the solution a the previous time step, \ref{ass:MPC:RPI-Set} and definition of the corresponding references.
	Using the same arguments it also holds $x(t+1)\in\mathbb{X}$ and $u(t)\in\mathbb{U}$.
	
	\ref{MPC:MPC:RobustConvergence} We use the previous candidate solution, \ref{ass:MPC:Ve} and standard \ac{MPC}-arguments \cite[Theorem 1]{Limon2010}.
	Furthermore, it holds $l_0(\tilde{\xi}_0-\bar{\xi}_0(t),\tilde{\xi}_{\mathrm{ref},0}(t) - \bar{\xi}_{\mathrm{ref},0})=0$ such that
	\begin{equation*}
		J^*(\xi(t+1))-J^*(\xi(t)) \leq \tilde{J}(\xi(t+1))-J^*(\xi(t)) \leq - l_0(\xi_0^*(t)-\bar{\xi}_0(t),\xi_{\mathrm{ref},0}^*(t) - \bar{\xi}_{\mathrm{ref},0})-l(\xi^*_0(t) - \xi^*_{\mathrm{ref},0}(t), u^*_0(t) - K_u \xi^*_{\mathrm{ref,0}}(t)).
	\end{equation*}
	As all cost terms are non-negative if follows
	\begin{align*}
		\lim\limits_{t\to\infty}l(\xi^*_0(t) - \xi*_{\mathrm{ref},0}(t), u^*_0 - K_u \xi^*_{\mathrm{ref},0}(t)) = 0\\
		\lim\limits_{t\to\infty}l_0(\xi_0^*(t)-\bar{\xi}_0(t),\xi_{\mathrm{ref},0}^*(t) - \bar{\xi}_{\mathrm{ref},0}) = 0
	\end{align*}
	Due to $Q\succeq 0$, $R\succ 0$, $(Q^{\tfrac{1}{2}}, \bar{A})$, we conclude that
	\begin{align*}
		\lim\limits_{t\to\infty} \xi^*_0(t) - \xi_{\mathrm{ref},0}^*(t) = 0 \\
		\lim\limits_{t\to\infty} u^*_0(t) - K_u\xi_{\mathrm{ref},0}^*(t) = 0
	\end{align*}
	Furthermore, we can choose $u^*_k(t) = K_u\xi_{\mathrm{ref},k}^*(t)$, and $x^*_k(t) = \xi_{\mathrm{ref},k}^*(t)$ to reduce all stage costs to zero such that $\lim\limits_{t\to\infty} J^*(\xi(t)) - V(M_e\xi_{\mathrm{ref},0}^*(t))=0$.
	As $J^*(\xi(t))$ is non-negative and non-increasing, if follows that $V(M_e\xi_{\mathrm{ref},0}^*(t))$ converges to a constant value and that we can always construct one optimizer $\xi_{\mathrm{ref},0}^*(t)=(\bar{A}+\bar{B}_u)\xi_{\mathrm{ref},0}^*(t-1)$ and $\xi_{0}^*(t)=\xi_{1}^*(t-1)$.
	
	Now, we show that $\lim\limits_{t\to\infty}M_e \xi^*_{\mathrm{ref},0}(t)-M_e \xi^\star(\xi^*_{\mathrm{ref},0}(t))=0$. 
	We can use similar arguments as in \cite[Lemma 1]{Limon2010} and use a proof by contradiction.
	Todo so, we consider the converged extended state $\xi^*_{\mathrm{ref},0}(t)=(\bar{A}+\bar{B}_uK_u)\xi^*_{\mathrm{ref},0}(t-1)$ and show that if $V(M_e\xi^*_{\mathrm{ref},0}(t))\neq V(M_e\xi^\star(\xi^*_{\mathrm{ref},0}(t))$ this can not be an optimal solution.
	We consider a new candidate solution $\xi^\circ$
	\begin{equation*}
		\xi^\circ_k = \beta \xi^*_{\mathrm{ref},k}(t) + (1-\beta)\xi^\star_k	\qquad \beta \in[0,1]
	\end{equation*}
	with $\xi^\star_k=(\bar{A}+\bar{B}_uK_u)^k\xi^\star(\xi^*_{\mathrm{ref},0}(t))$ being the corresponding reference trajectory.
	Due to the references being within the interior of the convex constraint sets, $(A,B)$ being controllable and \ref{ass:Setup:Sylvester}, there exists a $\hat{\beta}\in[0,1)$ such that for every $\beta\in[\hat{\beta},1)$ it is possible to find an input trajectory $\bar{u}$ to steer the system from $\xi^*_{\mathrm{ref},k}$ to $\xi^\circ_k$ in $\FB{insert minimum number of steps}$ steps.
	Furthermore, one can find an input trajectory such that the following holds
	\begin{equation*}
		l_0(\xi^*_0(t) - \xi_{\mathrm{ref},0}^*(t),\xi^\circ_0-\xi_{\mathrm{ref},0}^*(t)) + \sum_{k=0}^{N-1} l(\xi_k - \xi^\circ_k, u_k- \bar{u}_k) \leq \kappa \| \xi^*_{\mathrm{ref},0}(t) - \xi^\circ_0\|^2
	\end{equation*}
	for some $\kappa >0$.
	Hence, it holds
	\begin{equation*}
		\bar{J} \leq \kappa \| \xi^*_{\mathrm{ref},0}(t) - \xi^\circ_0\|^2 + V(M_e \xi^\circ_0).
	\end{equation*}
	Using convexity of $V$, it must further hold
	\begin{align*}
		\bar{J}-J^* = (1-\beta)^2 \kappa \| \xi^*_{\mathrm{ref},0}(t) - \xi^\star_0\|^2 + (1-\beta) (V(M_e\xi^\star_0) - V(M_e \xi^*_{\mathrm{ref},0}(t))) +  V(M_e \xi^\circ_0) \FB{Complete while looking up}
	\end{align*}
	As $V(M_e\xi^\star_0) - V(M_e \xi^*_{\mathrm{ref},0}(t))) < 0$, we can find a $\beta\in[\hat{\beta},1)$ such that $\bar{J}-J^*<0$. 
	This is contradiction to the optimal solution, hence we showed $\lim\limits_{t\to\infty}M_e\xi^*_{\mathrm{ref},0}(t) - M_e\xi^\star(\xi^*_{\mathrm{ref},0}(t)=0$.
	Lastly, we note that $C_e\xi(t)$ must lie within $C_e\xi^*_{\mathrm{ref},0}(t)\oplus C_e\mathbb{S}$.
	
	\ref{MPC:MPC:NominalConvergence} From \ref{MPC:MPC:RobustConvergence}, we know that that $M_e\xi_0^*(t)$ asymptotically converges to $M_e\xi^\star(\xi^*_{0}(t)$ and the control input follows $u(t)=K_u \xi^*_0(t) + K(\xi(t)-\xi^*_0(t))$.
	As $p(z)\{w(t)\}=0$, we conclude that $w(t)=w_{\mathrm{nom}}(t)$. 
	Applying the controller from \ref{ass:MPC:ZeroOffsetController} with $\eqref{eq:MPC:DeltaXi}$ also gives us asymptotic tracking of the corresponding $M_e\xi_0^*(t)$.
	
	\ref{MPC:MPC:Robustness} As $w(t)\in\mathrm{int}(\mathcal{W})$, it is possible to find a sufficiently small $\epsilon$ such that $w(t) + \bar{v}(t) - v(t)\in\mathcal{W}$ for all $t$.
	Hence, the change to $\bar{v}(t)$ can be represented using the disturbance, and feasibility remains.
\end{proof}
